# Supplementary material for: UQABench: Evaluating User Embedding for Prompting LLMs in Personalized Question Answering
Source: arXiv:2502.19178 source file (2025-04-01)
Supplement: Supplementary file 1 [file appendix.tex]

\section{Few-shot Prompt}
\label{sec:appendix}

\noindent\rule{0.45\textwidth}{0.4pt}
\begin{lstlisting}
Translate the following sentence by choosing the most appropriate option from the options to fill in the blank so that it complies with the logic and knowledge in the field of e-commerce and lifestyle consumption. Just output the chosen option. The bracket contains the tag of the phrase. Complete example 3 by imitating example 1 and example 2.

Example 1
Sentence: Rapid heating (function) is important for ___ (category)
Options: ['Microwave', 'Flashlight', 'Electric fan', 'Sound system']
Answer: Microwave

Example 2
Sentence: Keeping warm (function) is important for ___ (category)
Options: ['Short sleeve shirt', 'Down jacket', 'Slippers', 'Sun hat']
Answer: Down jacket

Example 3
Sentence: Babies (demographic) can be associated with or considered in relation to ___ (action)
Options: ['Listening to music', 'Painting', 'Studying', 'Reading']
Answer:
\end{lstlisting}
\noindent\rule{0.45\textwidth}{0.4pt}

\section{Prompt Designing}
\noindent\rule{0.45\textwidth}{0.4pt}
\begin{lstlisting}
Determine if the #answer# satisfies the #question#, first answer yes or no, then explain why.
#Question#
Choose the most appropriate option from the options to fill in the blank to complete the following sentence so that it aligns with the logic and knowledge in the e-commerce and lifestyle consumption fields. Just output the chosen option. The bracket contains the tag of the phrase.
Sentence: Babies (demographic) can be associated with or considered in relation to ___ (action)
Options: ['Painting', 'Studying', 'Reading', 'Drawing']
#Answer#
Studying
\end{lstlisting}
\noindent\rule{0.45\textwidth}{0.4pt}
